# Supplementary material for: Cyber-resilient Automatic Generation Control for Systems of AC Microgrids
Source: arXiv:2208.11163 source file (2023-04-25)
Supplement: Supplementary file 1 [file Appendix1.tex]

\section{Cyber Attack Detection Using Dynamic Watermarking Approach}
\label{sec:app_watermark}
This section illustrates the detailed procedure for cyber attack detection based on the watermarking approach. As illustrated in Figure \ref{fig:dynamic_watermark}, a watermark signal $\mathbf{e} \sim \mathcal{N}(0,\Sigma)$ is superposed in the control signal $\Delta \boldsymbol{\omega}_{\text{s}}$ produced by the secondary controller, where $\Sigma$ is the covariance matrix of $\mathbf{e}$. Denote by $\Delta\mathbf{P}_{\text{G}}'$ the measurements of the real power $\Delta\mathbf{P}_{\text{G}}$ that are received by the secondary frequency regulator. If there is no cyber attacks on $\Delta\mathbf{P}_{\text{G}}$, $\Delta\mathbf{P}_{\text{G}}' = \Delta\mathbf{P}_{\text{G}}$. With the true sequence of $\{\Delta \boldsymbol{\omega}_{\text{s}}[i]\}$ and $\{\mathbf{e}[i]\}$ for $i=0,1,\ldots, k-1$, one can approximately predict $\Delta\mathbf{P}_{\text{G}}[k]$ based on
\begin{subequations}\label{eq:PG_predict_whole}
    \begin{align}
        &\hat{\mathbf{x}}'[k] = A'\hat{\mathbf{x}}'[k-1] + B' \Delta \boldsymbol{\omega}_{\text{s}}[k-1] + \boldsymbol{e}[k-1]\label{eq:PG_predict1}\\
        &\Delta\hat{\mathbf{P}}_{\text{G}}[k] = C'\hat{\mathbf{x}}'[k] \label{eq:PG_predict2}
    \end{align}
\end{subequations}
where $\Delta\hat{\mathbf{P}}_{\text{G}}$ is the predicted version of $\Delta\mathbf{P}_{\text{G}}[k]$; and $\hat{\mathbf{x}}[k]$ is an intermediate variable which can be obtained by using \eqref{eq:PG_predict1} recursively. It can be observed from \eqref{eq:discrete_PG_prediction} that $\Delta\mathbf{P}_{\text{G}}$ cannot be exactly predicted due to the unavailability of $\hat{\mathbf{x}}'[0]$, $\Delta P_{\text{L}}'$ and $\mathbf{n}$. Define
\begin{equation}
    \boldsymbol{\nu}[k]:=\Delta\mathbf{P}_{\text{G}}'[k]-\Delta\hat{\mathbf{P}}_{\text{G}}[k].
\end{equation}

For a microgrid without cyber attack, i.e., $\Delta\mathbf{P}_{\text{G}}'[k] = \Delta\mathbf{P}_{\text{G}}[k]$, we can obtain a long sequence $\{\Delta\mathbf{P}'_{\text{G}}[k]|k=1, \ldots,W\}$ where $W$ is a large integer. The expectation $\boldsymbol{\mu}_{\nu}^*$ and covariance matrix $\Sigma_{\nu}^*$ of $\boldsymbol{\nu}$ in the microgrid without cyber attack can be approximated by $\hat{\boldsymbol{\mu}}_{\nu}^*$ and $\hat{\Sigma}_{\nu}^*$ where
\begin{subequations}
    \begin{align}
        &\hat{\boldsymbol{\mu}}_{\nu}^* = \frac{1}{W} \sum_{k=1}^W \boldsymbol{\nu}[k]\\
        &\hat{\Sigma}_{\nu}^* =\frac{1}{W}\sum_{k=1}^W (\boldsymbol{\nu}[k]-\hat{\boldsymbol{\mu}}_{\nu}^*)(\boldsymbol{\nu}[k]-\hat{\boldsymbol{\mu}}_{\nu}^*)^{\top}.
    \end{align}
\end{subequations}

For the microgrid that might be under cyber attacks where $\Delta\mathbf{P}_{\text{G}}'[k]$ may not be equal to $\Delta\mathbf{P}_{\text{G}}[k]$, denote by $\hat{\boldsymbol{\mu}}_{\nu}$ and $\hat{\Sigma}_{\nu}$ the estimated expectation and covariance matrix of $\boldsymbol{\nu}$, respectively. Let $\mathcal{M}_{\rho}$ collect $\Delta\mathbf{P}'$ from time $t=(\rho-W+1)\Delta t$ to $t=\rho\Delta t$, viz.,
\begin{equation}
    \mathcal{M}_{\rho}:= \{\Delta\mathbf{P}'_{\text{G}}[k]|k=\rho-W+1, \ldots,\rho\}.
\end{equation}
$\hat{\boldsymbol{\mu}}_{\nu}$ and $\hat{\Sigma}_{\nu}$ can be computed by 
\begin{subequations} \label{eq:estimation}
    \begin{align}
        &\hat{\boldsymbol{\mu}}_{\nu} = \frac{1}{W}\sum_{k=\rho-W+1}^{\rho} \boldsymbol{\nu}[k] \label{eq:mu_hat}\\
        &\hat{\Sigma}_{\nu} =\frac{1}{W}\sum_{k=\rho-W+1}^{\rho} (\boldsymbol{\nu}[k]-\hat{\boldsymbol{\mu}}_{\nu})(\boldsymbol{\nu}[k]-\hat{\boldsymbol{\mu}}_{\nu})^{\top}. \label{eq:sigma_hat}
    \end{align}
\end{subequations}
If $\Delta\mathbf{P}_{\text{G}}'[k] = \Delta\mathbf{P}_{\text{G}}[k]$, $\hat{\boldsymbol{\mu}}_{\nu}$ and $\hat{\Sigma}_{\nu}$ should be close to $\hat{\boldsymbol{\mu}}_{\nu}^*$ and $\hat{\Sigma}_{\nu}^*$, respectively, that is,
\begin{subequations} \label{eq:two_conditions}
    \begin{align}
        &\xi_1 =\norm{\hat{\boldsymbol{\mu}}_{\nu}-\hat{\boldsymbol{\mu}}_{\nu}^*}_2 < \epsilon_1 \label{eq:cdt1}
        \\
        &\xi_2 = |\text{tr}(\hat{\Sigma}_{\nu}-\hat{\Sigma}_{\nu}^*)|<\epsilon_2
        \label{eq:cdt2}
    \end{align}
\end{subequations}
where $\norm{\cdot}_2$ and $\text{tr}(\cdot)$ are the $\mathcal{L}_2$ norm and the trace operator, respectively; and $\epsilon_1$ and $\epsilon_2$ are positive numbers. Violation of either \eqref{eq:cdt1} or \eqref{eq:cdt2} or both suggests cyber attacks, i.e., $\Delta\mathbf{P}_{\text{G}}[k]\ne \Delta\mathbf{P}'_{\text{G}}[k]$. The two conditions in \eqref{eq:two_conditions} can be checked in a moving-window fashion, which is summarized in Algorithm \ref{alg:1}. Function \texttt{DW} in Algorithm \ref{alg:1} returns a binary result: $0$ suggests a cyber attack is not detected, while $1$ suggest no cyber attack is detected.

%we can estimate the expectation $\boldsymbol{\mu}_{\nu}^*$ and covariance matrix $\Sigma_{\nu}^*$ of $\boldsymbol{\nu}$ by obtaining a long sequence of $\{\mathbf{\Delta\mathbf{P}'_{\text{G}}}[k]|k=0, \ldots,W\}$.
%If there is no cyber attack, i.e., $\Delta\mathbf{P}_{\text{G}}'[k] = \Delta\mathbf{P}_{\text{G}}[k]$, we can estimate the 
%Denote by $\boldsymbol{\mu}_{\nu}^*$ and $\Sigma_{\nu}^*$ the mean and covariance matrix of $\boldsymbol{\nu}$ 

\begin{algorithm}
    \caption{Watermarking-based Cyber Attack Detection} \label{alg:1}
        \begin{algorithmic}[1]
            \Function{\tt DW}{$\mathcal{M}_{\rho-1}$, $\Delta \mathbf{P}_{\text{G}}'[\rho]$}
                \State $\mathcal{M}_{\rho} \leftarrow \left\{\Delta \mathbf{P}_{\text{G}}'[\rho]\right\} \cup \mathcal{M}_{\rho-1} -\left\{\Delta \mathbf{P}_{\text{G}}'[\rho-W]\right\}$
                \State Compute $\nu_{\rho-W+1}, \ldots,\nu_{\rho}$ based on $\mathcal{M}_{\rho}$ and \eqref{eq:PG_predict_whole}
                \State Compute $\hat{\boldsymbol{\mu}}_{\nu}$ and $\hat{\Sigma}_{\nu}$ based on \eqref{eq:estimation}
                \State Obtain $\xi_1$ and $\xi_2$ according to \eqref{eq:two_conditions}
                \If{$(\xi_1<\epsilon_1)\land (\xi_2<\epsilon_2)$}
                \State \Return $0$ \algorithmiccomment{No attack is detected}
                \Else \State \Return $1$ \algorithmiccomment{Attack is detected}
                \EndIf
            \EndFunction
        \end{algorithmic}
\end{algorithm}

\section{Overall Procedure of Cyber-resilient Frequency Regulation} \label{app:summary}
Algorithm \ref{alg:2} summarizes the overall procedure described in Sections \ref{sec:SectionIII} and \ref{sec:cyber_attack}. Line $3$ of Algorithm \ref{alg:2} is relevant to cyber attack detection which is described in Section \ref{subs: cyber_attack_detection}; Line $4$ is described in Section \ref{subs:OFR}; Lines $6$-$8$ are presented in Section \ref{ssubsec: observer}; and Lines $10$-$11$ are presented in Section \ref{subsubs:networked}.
\begin{algorithm}
    \caption{Cyber Resilient $\mu$AGC} \label{alg:2}
        \begin{algorithmic}[1]
        \State $\mathcal{M}_W \leftarrow \cup_{k=1}^W \{\Delta \mathbf{P}_{\text{G}}'[k]\}$
        \While{$\rho = W+1, W+2, \ldots$}
            \If{$\texttt{DW}(\mathcal{M}_{\rho-1}, \Delta \mathbf{P}_{\text{G}}'[\rho])=0$}
            \State Compute $\Delta \boldsymbol{\omega}_{\text{s}}[\rho]$ via \eqref{eq:z_i_int} and \eqref{eq:Kz}
            \Else
            \If{Neighboring microgrids are unavailable}
            \State Compute $\Delta \boldsymbol{\omega}_{\text{s}}[\rho]$ via \eqref{eq:P_G_observer} and \eqref{eq:Kz_hat}. \State $\mathbf{e}[\rho]\leftarrow0$ \algorithmiccomment{Stop injecting watermark}
            \Else
            \State $\Delta \boldsymbol{\omega}_{\text{s}}[\rho]\leftarrow 0$; $\mathbf{e}[\rho]\leftarrow0$
            %\algorithmiccomment{Disable secondary control}
            \State Network with the neighboring microgrids
            \EndIf
            \EndIf
        \State\Return $\Delta \boldsymbol{\omega}_{\text{s}}[\rho]$
        \EndWhile
        \end{algorithmic}
\end{algorithm}
